# Supplementary material for: A simple DNN regression for the chemical composition in essential oil
Source: arXiv:2412.12936 source file (2024-12-17)
Supplement: Supplementary file 1 [file SupInfo.pdf]

# (SUPPORTING INFORMATION FOR) A SIMPLE DNN REGRESSION FOR THE CHEMICAL COMPOSITION IN ESSENTIAL OIL

A PREPRINT

**Yuki Harada**
Priority Organization for Innovation and Excellence Laboratory for Data Sciences,
Kumamoto University, Kurokami 2-39-1, Chuo-ku, Kumamoto 860-8555, JP
yharada@kumamoto-u.ac.jp

**Shuichi Maeda**
Priority Organization for Innovation and Excellence Laboratory for Data Sciences,
Kumamoto University, Kurokami 2-39-1, Chuo-ku, Kumamoto 860-8555, JP
Shuichi2503736@gmail.com

**Masato Kiyama**
Faculty of Advanced Science and Technology,
Kumamoto University, Kurokami 2-39-1, Chuo-ku, Kumamoto 860-8555, JP
masato@cs.kumamoto-u.ac.jp

**Shinichiro Nakamura**
Priority Organization for Innovation and Excellence Laboratory for Data Sciences,
Kumamoto University, Kurokami 2-39-1, Chuo-ku, Kumamoto 860-8555, JP
shindon@kumamoto-u.ac.jp

December 16, 2024

## 1 Experiments

### 1.1 (SI) Difficulty in accurate quantification of gas chromatography (GC)

In ideal conditions in GC, the area% of a peak is proportional to the weight content of the component,several factors can shift this relationship: Including Response Factors (Relative Sensitivity, sometime found in FID, TCD), Saturation or Non-Linear Response in Detector, Sample Matrix Effects, Volatility and Thermal Decomposition mainly in injection or in column, and, Instrumental and Method Errors such as Baseline noise or peak separation difficulty. To ensure accurate quantification of the target molecule, calibration standards are widely used to determine individual response factors. Kumar et al. [2018]

### 1.2 (SI) Cross-validation and Predictability

We run k-fold cross-validation procedure to evaluate your classifier/model. For each iteration (fold) of cross-validation, we acquired the predicted probabilities for each instance in the validation set. After completing all folds of cross-validation, we created the ROC curve and calculated the true positive rate (TPR) and false positive rate (FPR). We produced the ROC curve and then calculated the AUC using the predicted scores and true labels (ground truth) from the validation set. The area under the ROC curve (AUC) assesses the classifier's overall prediction performance across all classification levels.

KfoldCV in Sklearn was used to do 5 fold cross-validation in the regression. Fig.(S)1 shows this procedure the cross-validation and AUC calculations for each descriptor.

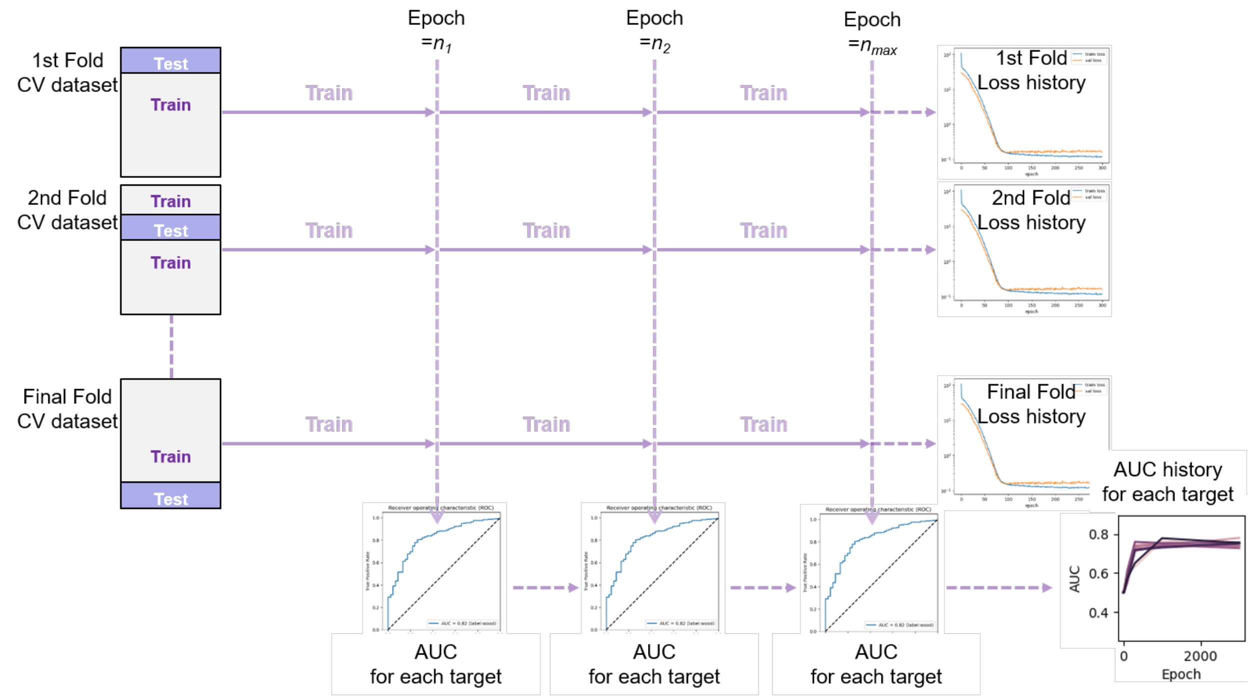


Figure 1: The procedure of cross-validation and AUC calculations for each descriptor

## 2 Disuccusion

### 2.1 (SI) Prediction performance in other conditions

Prediction performance by 3 DNN and 2 loss function were obtained as shown in Fig.(S)2-7:

## 3 (SI) Future Task

### 3.1 (SI) Note for "Olfactory Label Prediction on Aroma-Chemical Pairs"

We will disuccuss about 'boldly design of the whole chemical space as a perspective using graph neural network' by sisson et.al. [Sisson et al., 2023, et. al.] for chemical space investigation. This hypergraph-based worldview is similar to the relational analysis of a friend-network on social media. The edges (relationships between nodes) in the hypergraph are concatenated odor characteristics, which is also an innovative concept. However, staying on a single hypergraph and attempting edge design with odor characteristics results in a difficulty beyond our imagination, when "incorporating concentration information into nodes of hypergraph" and/or "building blends of more than two" as Sisson noted. "Incorporating concentration information" may be achievable by modifying the node design of the hypergraph, but preparing for adequate sensory evaluation would necessitate a large number of psychological experiments.

Our future interest include understanding the true nature of the vector representation (embedding) in the whole chemical space other than the molecular structural representation (embedding), as well as developing the design relevant to properties of chemical. The validity of our interest cannot be assessed at this time. We currently give up on using odor characters as the objective variable due to insufficient data for study (as noted by Sisson). Sisson mentions the future task of using innovative techniques and novel estimation procedures for sparse datasets, and we agree.

## References

Yogesh Kumar, Om Prakash, Himanshu Tripathi, Sudeep Tandon, Madan M Gupta, Laiq-Ur Rahman, Raj K Lal, Manoj Semwal, Mahendra Pandurang Darokar, and Feroz Khan. Aromadb: a database of medicinal and aromatic plant's aroma molecules with phytochemistry and therapeutic potentials. *Frontiers in plant science*, 9:1081, 2018.

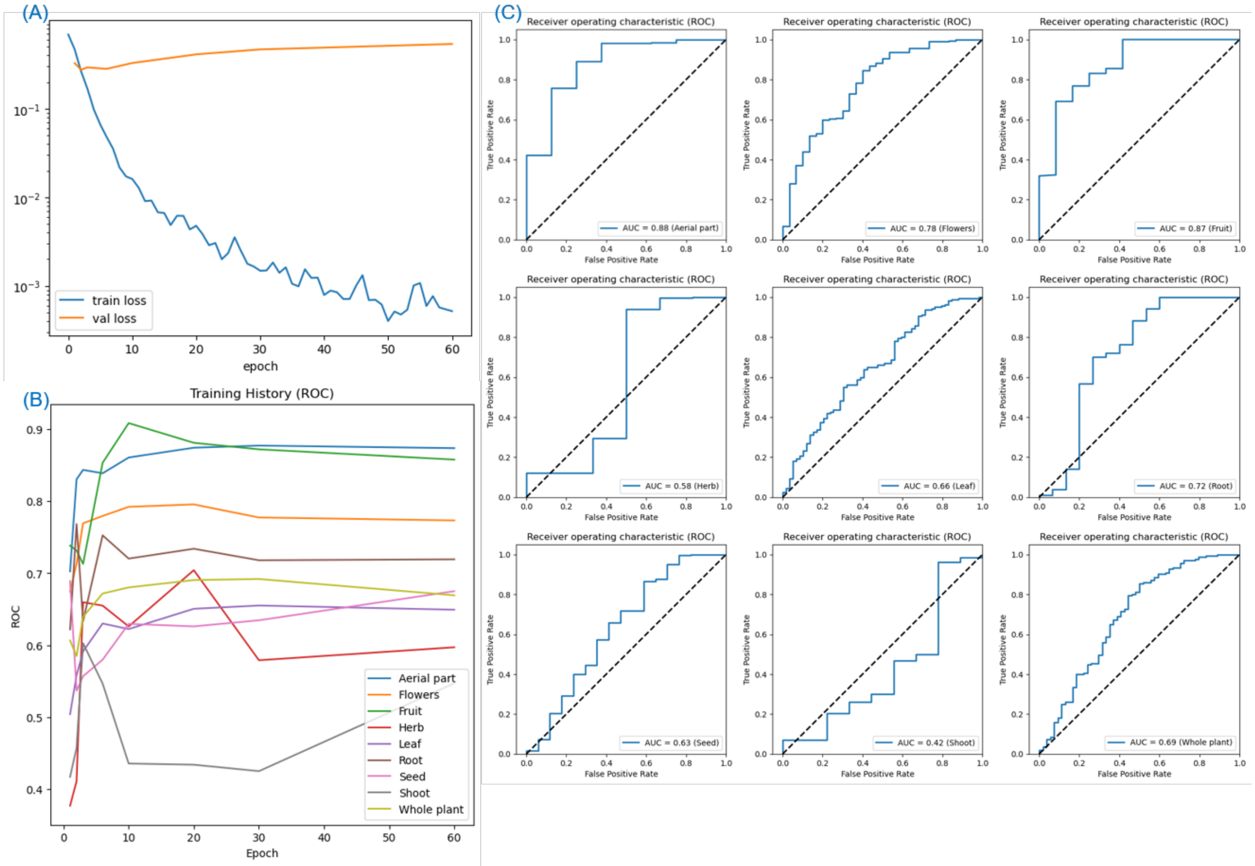


Figure 2: Prediction performance by CNN with NLL (1st entry in Table 02) (A) Train loss vs epochs, (B) Test AUC vs epochs, and (C) ROC plot (epoch=30) for each target

Laura Sisson, Aryan Amit Barsainyan, Mrityunjay Sharma, and Ritesh Kumar. Olfactory label prediction on aroma-chemical pairs. *arXiv preprint arXiv:2312.16124*, 2023.

Laura Sisson et. al. Github - odor-pair. `https://github.com/odor-pair/odor-pair`.

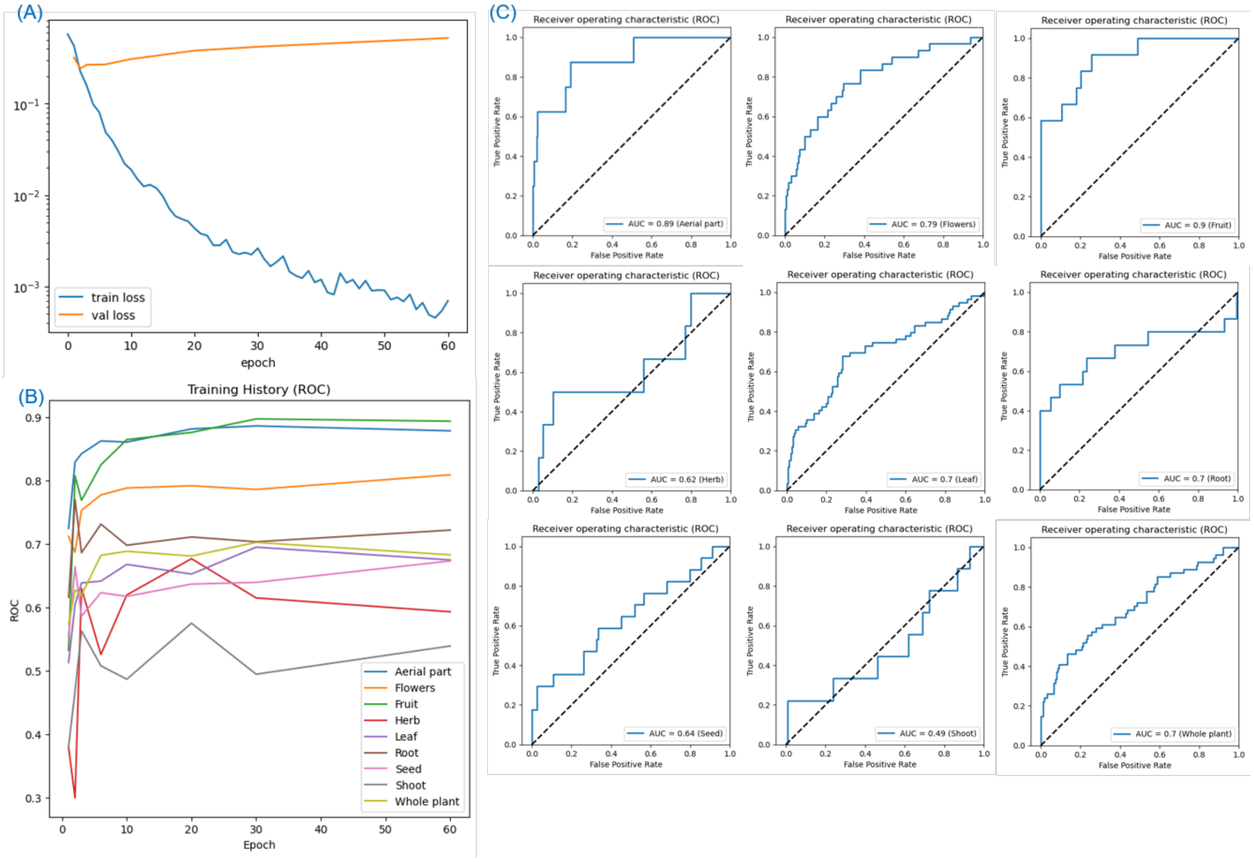


Figure 3: Prediction performance by CNN with BCE logit loss (2nd entry in Table 02) (A) Train loss vs epochs, (B) Test AUC vs epochs, and (C) ROC plot (epoch=30) for each target

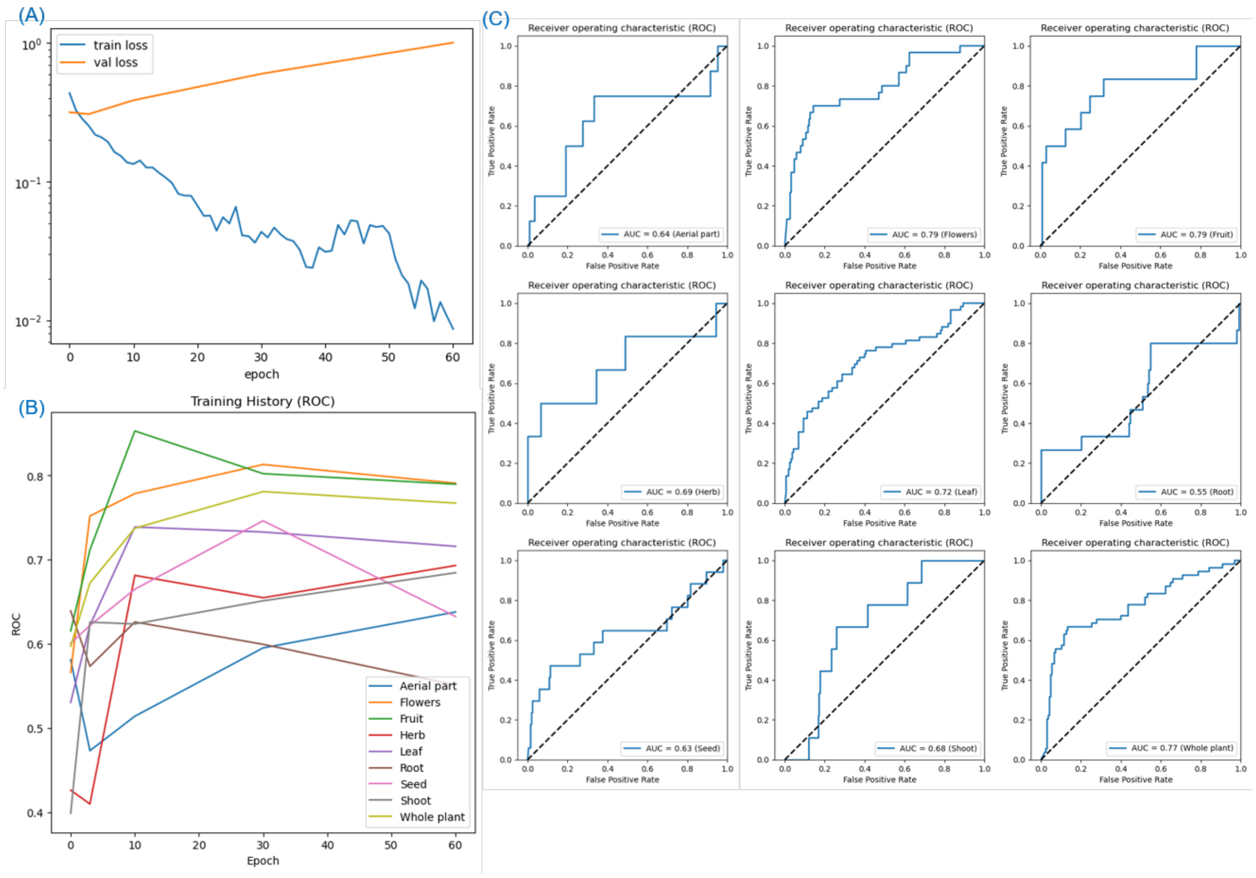


Figure 4: Prediction performance by GCN with NLL (3rd entry in Table 02) (A) Train loss vs epochs, (B) Test AUC vs epochs, and (C) ROC plot (epoch=30) for each target

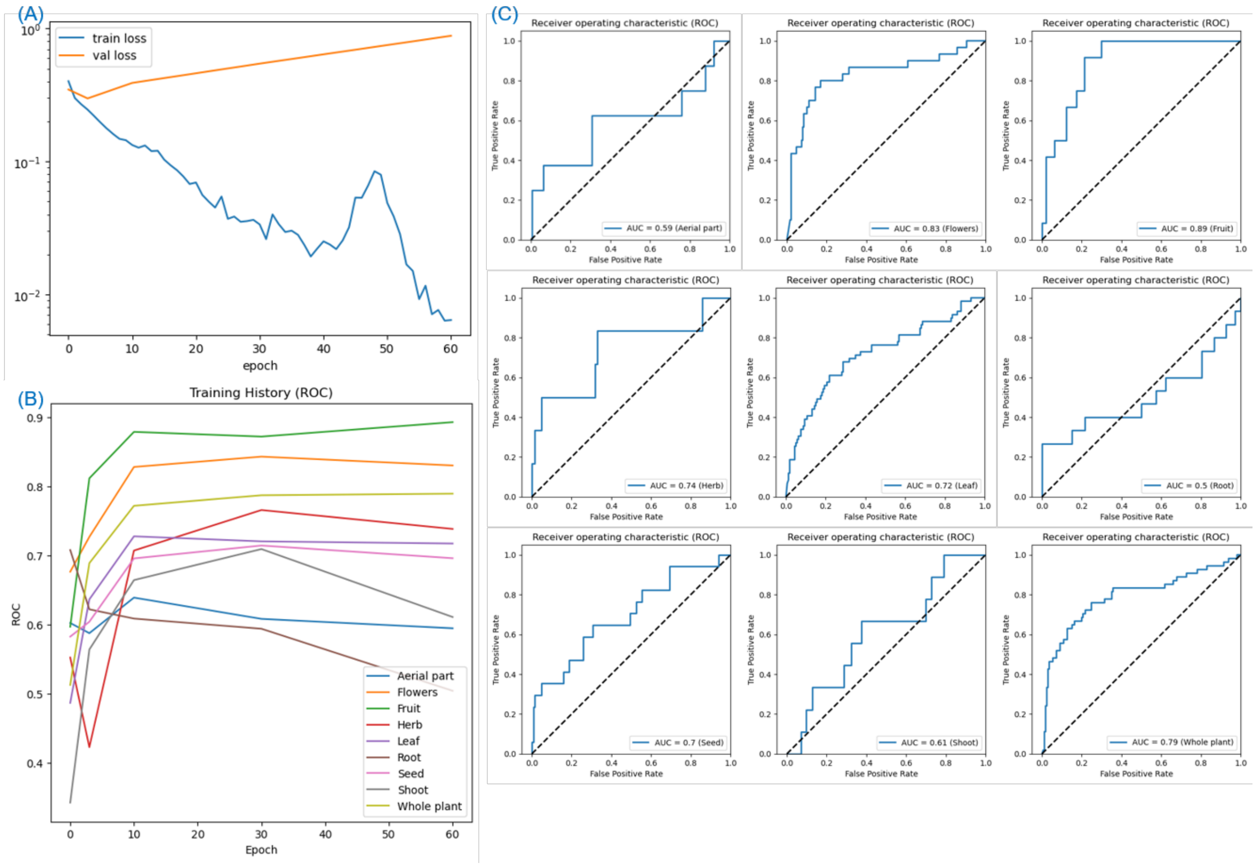


Figure 5: Prediction performance by GCN with BCE logit loss (4th entry in Table 02) (A) Train loss vs epochs, (B) Test AUC vs epochs, and (C) ROC plot (epoch=30) for each target

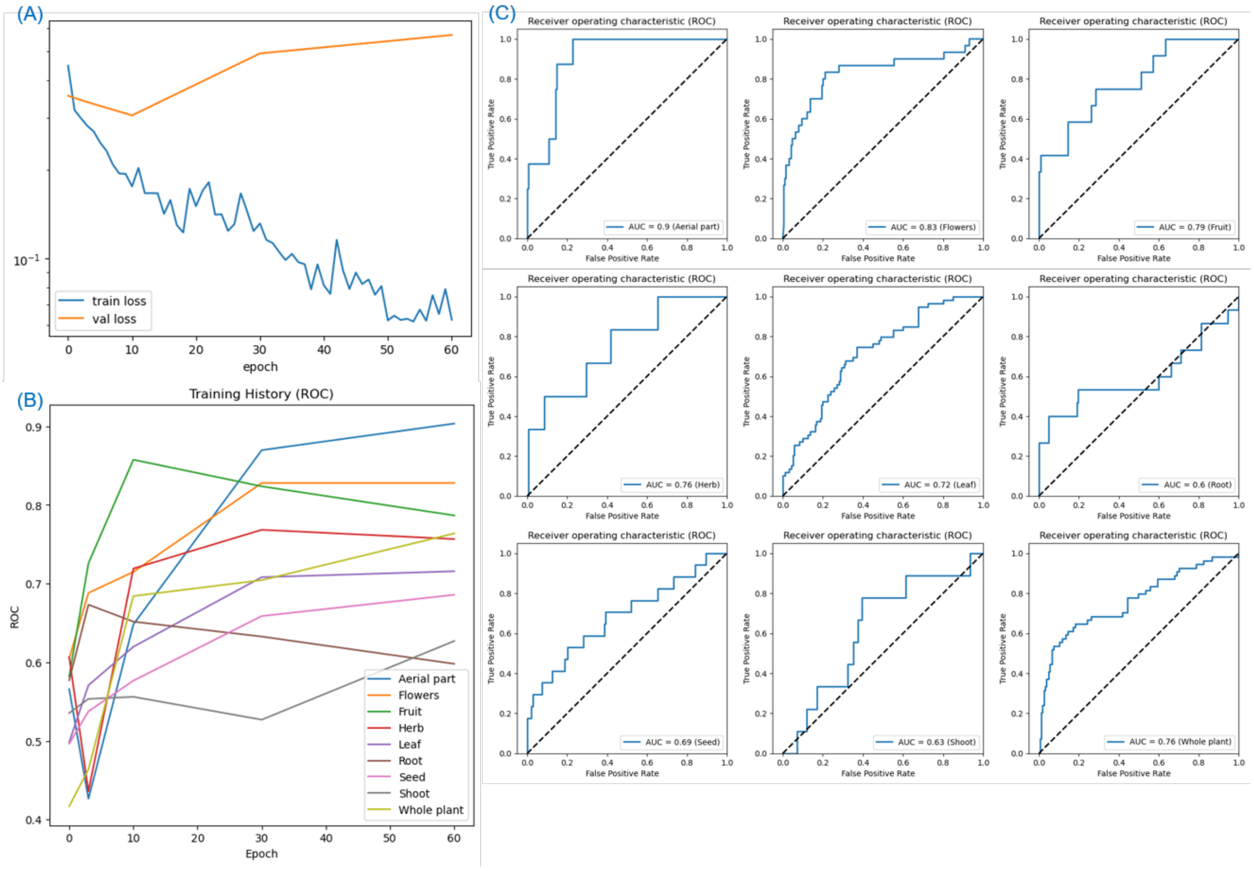


Figure 6: Prediction performance by GAT with NLL (5th entry in Table 02) (A) Train loss vs epochs, (B) Test AUC vs epochs, and (C) ROC plot (epoch=30) for each target

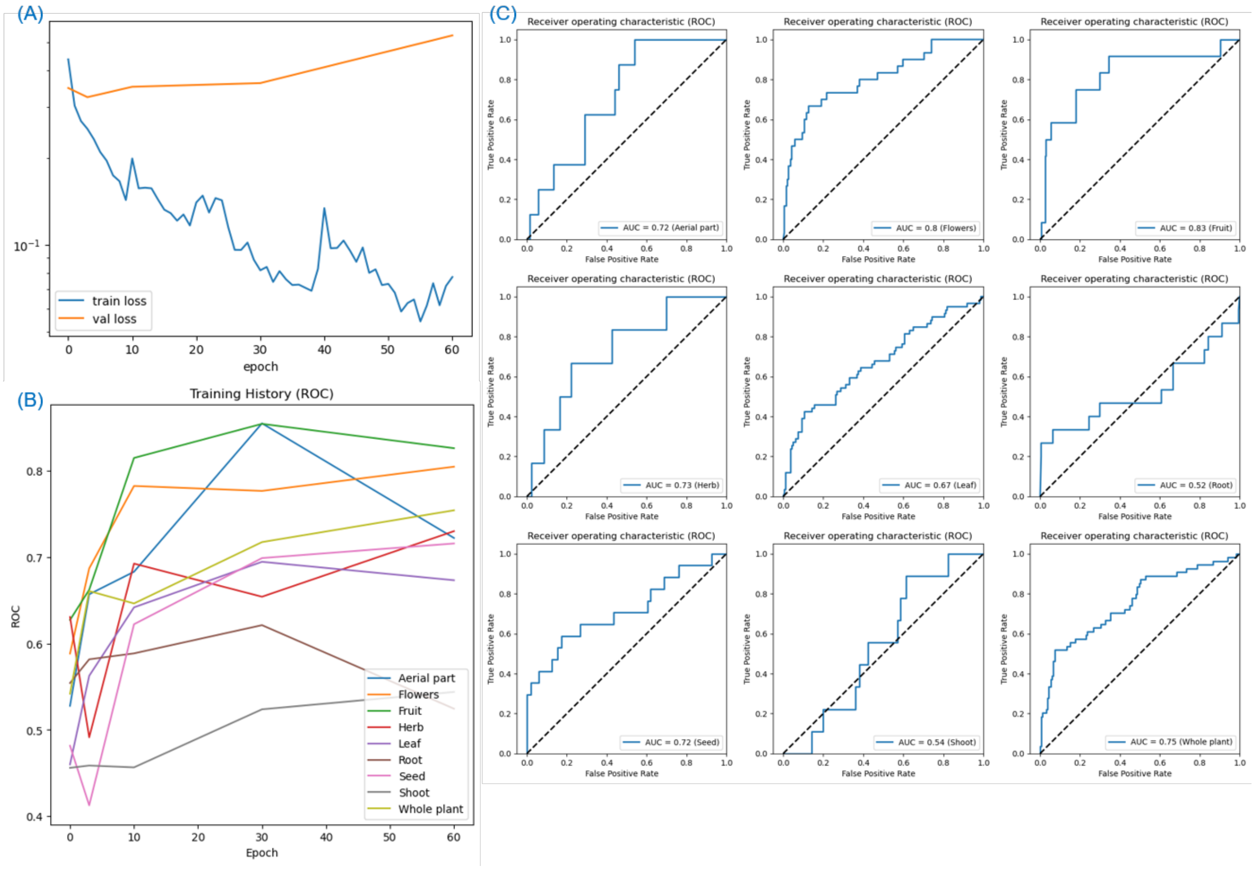


Figure 7: Prediction performance by GAT with BCE logit loss (6th entry in Table 02) (A) Train loss vs epochs, (B) Test AUC vs epochs, and (C) ROC plot (epoch=30) for each target
